# Supplementary material for: Modeling of Ballistic Electron Emission Microscopy on metal thin films
Source: arXiv:1501.06458 source file (2015-01-26)
Supplement: Supplementary file 2 [file apl.pdf]

AIP Applied Physics Letters

# k-space spin filtering effect in the epitaxial Fe/Au/Fe/GaAs(001) spin-valve

M. Hervé, S. Tricot, Y. Claveau, G. Delhaye, B. Lépine, S. Di Matteo, P. Schieffer, and P. Turban

Citation: Applied Physics Letters **103**, 202408 (2013); doi: 10.1063/1.4831755
View online: http://dx.doi.org/10.1063/1.4831755
View Table of Contents: http://scitation.aip.org/content/aip/journal/apl/103/20?ver=pdfcov
Published by the AIP Publishing

AIP Publishing Re-register for Table of Content Alerts

Create a profile. Sign up today!

This article is copyrighted as indicated in the abstract. Reuse of AIP content is subject to the terms at: http://scitation.aip.org/termsconditions. Downloaded to IP: 129.20.76.104 On: Wed, 20 Nov 2013 10:07:47

APPLIED PHYSICS LETTERS **103**, 202408 (2013)

# k-space spin filtering effect in the epitaxial Fe/Au/Fe/GaAs(001) spin-valve

M. Hervé, S. Tricot, Y. Claveau, G. Delhaye, B. Lépine, S. Di Matteo, P. Schieffer, and P. Turban[a)]
*Département Matériaux et Nanosciences, Institut de Physique de Rennes, UMR 6251, CNRS-Université de Rennes 1, Campus de Beaulieu, Bât 11E, 35042 Rennes cedex, France*

(Received 11 October 2013; accepted 3 November 2013; published online 14 November 2013)

The hot-electron magnetotransport of epitaxial Fe/Au/Fe/GaAs(001) spin-valves is investigated by ballistic-electron magnetic microscopy. A magnetocurrent amplitude larger than 500% is observed at room temperature close to the Schottky barrier energy. Remarkably, this magnetocurrent is not significantly affected by the thickness reduction of ferromagnetic films, down to 5 atomic layers of the Fe(001) top electrode. This rather suggests a dominant interfacial spin-filtering effect. Finally, the magnetocurrent is strongly reduced when the effective mass of the semiconductor collector is increased. These observations are consistent with recent theoretical prediction of k-space spin-filtering effect in epitaxial spin-valves attached to a semiconducting lead. © *2013 AIP Publishing LLC*. [http://dx.doi.org/10.1063/1.4831755]

During the last decade, the introduction of epitaxial MgO tunnel barrier in magnetic tunnel junctions[1–4] has allowed record tunneling magnetoresistance (TMR) ratios at room temperature, opening the way to industrial-scale devices such as TMR-based magnetic reading heads or magnetic random access memories.[5] In Fe/MgO/Fe(001) magnetic tunnel junctions, this giant TMR effect is well described by first-principle theories[6,7] and originates from a coherent spin-dependent tunneling of highly spin-polarized Fe $\Delta_1$ Bloch states close to the Fermi energy in the parallel wave vector $k_{\parallel} = 0$ direction. Further recent calculations by Autès and coworkers[8] suggested that even higher magnetoresistance (MR) amplitude could be achieved in fully metallic Fe/Ag/Fe(001) epitaxial spin-valve attached to a semiconductor lead. Briefly, the use of a n-doped semiconducting lead with a very small Fermi surface allows selecting electrons with a $k_{\parallel}$ very close to the $\bar{\Gamma}$ point, acting thus as a collimator. In this particular k-space direction, a good match between Fe and Ag $\Delta_1$ bands is observed for majority-spin electrons while minority-spin electrons are fully reflected at the Fe/Ag interface resulting in a vanishing conductance in the antiparallel magnetic configuration of the spin-valve.

In this letter, we investigate by ballistic electron magnetic microscopy (BEMM) the hot-electron magnetotransport properties of Fe/Au/Fe(001) spin-valves epitaxially grown on n-doped GaAs(001) and $Al_xGa_{1-x}As(001)$ semiconducting layers. We limited ourselves to ultrathin metallic spin-valves with a total Fe thickness smaller than 2.9 nm. On the one hand, we observe a large magnetoconductance effect, almost independent of the top Fe electrode thickness down to 5 atomic planes, suggesting a dominant interfacial spin-filtering effect. On the other hand, the magnetoconductance amplitude is largely reduced while increasing the effective mass of the semiconductor lead, i.e., while increasing the semiconducting collimator radius. These experimental observations are consistent with the theoretical predictions of Autès *et al.*[8] and open the way to large magnetoresistance ratios by combining engineered epitaxial spin-valves and a semiconducting drain.

The Au(2.2 nm)/Fe(0.7–1.7 nm)/Au(2.6 nm)/Fe(1.2 nm)/GaAs(001) spin-valves are deposited by molecular beam epitaxy (MBE). A 1.5 $\mu$m thick Si n-doped ($4 \times 10^{16}$ cm$^{-3}$) GaAs buffer layer is first grown in a independent MBE chamber on a $n^+$-GaAs(001) substrate. The whole semiconducting stack is protected by a 5 $\mu$m thick amorphous As capping layer to allow the transfer under ambient atmosphere in the BEMM setup. In the ultra-high vacuum (UHV) BEMM setup, thermal desorption of the As protecting layer is first done at 760 K in front of a cryopanel cooled with liquid nitrogen, leading to the formation of a clean As($2 \times 4$)-reconstructed GaAs(001). After sample cooling down to room temperature, the metallic spin-valve is deposited through a shadow mask to form 400 $\mu$m diameter metallic dots on the semiconducting substrate. Further details on samples growth can be found elsewhere.[9] In the following, all crystalline directions will refer to crystal directions of the GaAs(001) substrate. Electrochemically etched W STM tips are cleaned *in situ* by thermal heating before the BEMM experiments. A gold wire is used to ground the 400 $\mu$m diameter isolated metallic dots. All STM/BEMM experiments are performed at room-temperature in the constant-current mode of operation with a tunneling current set to $I_T = 20$ nA.

In a BEMM experiment,[10,11] the STM tip is used to inject locally a hot-electron current at the surface of the spin-valve, with an energy above the Fermi level defined by the tip bias value $U_{gap}$. A small part of the injected hot-electrons travels ballistically through the various layers and interfaces of the spin-valve and reaches the Fe/semiconductor interface. These ballistic electrons can finally enter the semiconductor conduction band (CB), provided their energy overcomes the Schottky barrier $\Phi_{SB}$ at the Fe/semiconductor interface. This ballistic current $I_C$ is collected at the back of the semicondutor substrate using an indium ohmic contact. $I_C$ depends on the relative magnetization orientation of the ferromagnetic electrodes of the spin-valve via the hot-electron giant MR effect. The inset of Figure 1(a) presents a typical $I_C(B)$ hysteresis loop recorded on a Au(2.2 nm)/Fe(1 nm)/Au(2.6 nm)/Fe(1.2 nm)/GaAs(001)

[a)]Author to whom correspondence should be addressed. Electronic mail: pascal.turban@univ-rennes1.fr

 © 2013 AIP Publishing LLC

This article is copyrighted as indicated in the abstract. Reuse of AIP content is subject to the terms at: http://scitation.aip.org/termsconditions. Downloaded to IP: 129.20.76.104 On: Wed, 20 Nov 2013 10:07:47

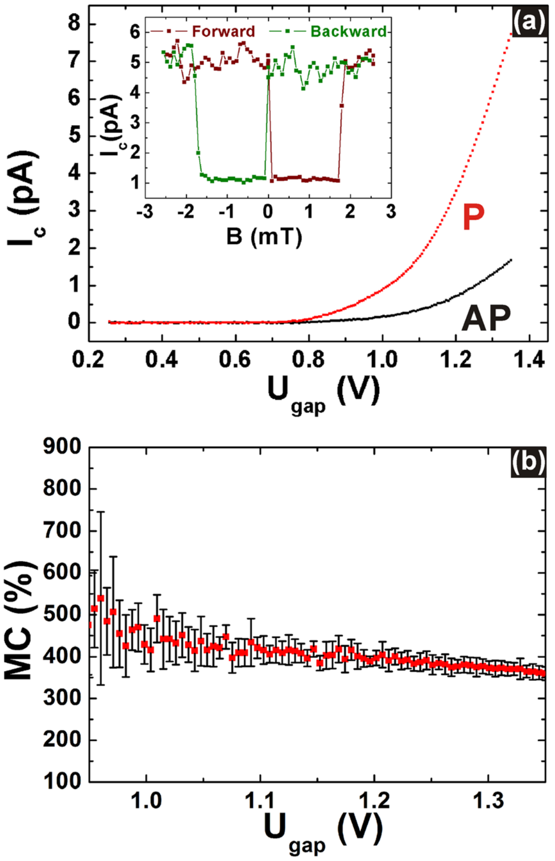


FIG. 1. (a) Ballistic electron spectroscopy curves $I_C(U_{gap})$ recorded on a Au(2.2 nm)/Fe(1 nm)/Au(2.6 nm)/Fe(1.2 nm)/GaAs(001) spin-valve in the parallel (red curve) and anti-parallel (black curve) magnetic configuration. Tunneling current was set to 20 nA. The inset displays a typical hysteresis loop $I_C(B)$ recorded at 1.25 eV of electron energy. The in-plane magnetic field was applied along the [110] direction. (b) Calculated magnetocurrent versus electron energy deduced from Figure 1(a).

spin-valve. $U_{gap}$ was set to 1.25 V and the in-plane magnetic field was swept along the [110] direction of the substrate, i.e., along a magnetic easy axis for both Fe electrodes. Two levels of collector current $I_C$ are observed: a large $I_C$ value ($Ic_{max} = 5$ pA) corresponding to the parallel configuration and a low $I_C$ value ($Ic_{min} = 1$ pA) corresponding to the antiparallel configuration of the spin-valve. The corresponding hot-electron magnetocurrent defined as follows: $MC^* = \frac{Ic_{max} - Ic_{min}}{Ic_{min}}$ is of 400% for electron energy of 1.25 eV. Figure 1(a) also displays the hot-electron spectroscopy curves $I_C(U_{gap})$ measured in the parallel (red curve) and antiparallel (black curve) magnetic configurations. 2000 individual $I_C(U_{gap})$ curves were averaged over a $500 \times 500$ nm$^2$ area in order to improve the signal-to-noise ratio. The collector current presents an onset at $U_{gap} = 0.76$ V corresponding to the Schottky barrier height $\Phi_{SB} = 0.76$ eV at the Fe/GaAs(001) interface.[12] From these curves, the energy dependence of the magnetocurrent can be calculated and is plotted on Figure 1(b). The MC error bars were calculated from the experimental standard deviation values observed over the two sets of 2000 individual $I_C(U_{gap})$ curves recorded in the parallel and antiparallel magnetic configuration. MC decreases from 500% to 360% in the 0.95 eV–1.35 eV energy range. Although the signal-to-noise ratio is weak at low energy in BEMM experiments, MC presents a tendency to increase faster below 1 eV, close to the Schottky barrier, as observed in equivalent solid-state devices operating with higher injection current such as the magnetic tunnel transistor.[13] In the following, we will further discuss the potential origin of these large magnetoconductance effects in such epitaxial spin-valve.

In BEMM experiments, the non magnetic STM tip injects unpolarized hot electrons at the spin-valve surface. The observed hot-electron magnetoresistance effect results from:[14] (i) spin-dependent scattering in the bulk of the ferromagnetic electrode; (ii) spin-dependent transmission coefficient for the hot-electrons at the interfaces, arising from band-structure matching. The latter effect can be dominant in ultrathin epitaxial samples[12] and may result in very large magnetoconductance effects.[8] In order to discriminate between bulk and interface spin-filtering effects in our epitaxial spin-valves, we have investigated the MC dependence with ferromagnetic layer thickness. The bottom Fe electrode ($Fe_1$) thickness was kept constant at 1.2 nm. For this thickness, the strong uniaxial magnetic anisotropy at the Fe/GaAs(001) interface defines a magnetic easy axis along the [110] direction.[15] The top Fe electrode ($Fe_2$) thickness was successively set to 0.7, 1, and 1.7 nm, corresponding to 5, 7, and 12 Fe(001) monoatomic layers (MLs), respectively. Magnetoresistive behaviours similar to Figure 1 were observed for the three samples and the corresponding raw magnetocurrent values MC* at 1.3 eV are reported in Table I.

In this $Fe_2$ thickness range, the magnetic anisotropy of the top Au/Fe/Au(001) ferromagnetic electrode is highly thickness-dependent.[16] For the 0.7 and 1 nm thick $Fe_2$ layers, we have checked by magneto-optical Kerr effect and diffusive four point probe magnetotransport measurements that $Fe_2$ was uniaxial with a magnetic easy axis parallel to [110]. For the 1.7 nm thick $Fe_2$ layer, we observed two easy axis located 39.5° away from the [110] direction. These observations are in agreement with results from literature.[16] As a consequence, the MC* values obtained for the spin-valves with a 0.7 and 1 nm thick $Fe_2$ layers correspond to a 0°–180° variation of the relative angle $\theta$ between $Fe_1$ and $Fe_2$ magnetizations. On the other hand, the MC* value obtained for the 1.7 nm thick $Fe_2$ layer corresponds to a reduced $\theta$ variation between 39.5° and 140.5°, i.e., for a $Fe_2$ magnetization jump between its two easy axis directions. The sudden decrease of MC* from 370% to 220% while increasing the $Fe_2$ thickness from 1 to 1.7 nm is thus due to the evolution of the magnetic anisotropy of the top electrode. In order to allow a direct comparison between the three investigated samples, we corrected the raw magnetocurrent MC* from these magnetic anisotropy variations by using a $\sin^2\left(\frac{\theta}{2}\right)$ angular dependence of the hot-electron current.[9,17] The normalized magnetocurrent values $MC_{180}$, calculated for a 0°–180° variation of $\theta$ are given in Table I. These measurements point out two main

TABLE I. Evolution of the magnetocurrent for various $Fe_2$ top electrode thickness.

| $Fe_2$ thickness | 0.7 nm/5 ML | 1 nm/7 ML | 1.7 nm/12 ML |
|---|---|---|---|
| $\Delta\theta$ | 180° | 180° | 100° |
| $MC^*$ at 1.3 eV | 320 ± 30% | 370 ± 30% | 220 ± 30% |
| $MC_{180}$ at 1.3 eV | 320 ± 30% | 370 ± 30% | 420 ± 30% |

This article is copyrighted as indicated in the abstract. Reuse of AIP content is subject to the terms at: http://scitation.aip.org/termsconditions. Downloaded to IP: 129.20.76.104 On: Wed, 20 Nov 2013 10:07:47

striking features: (i) $MC_{180}$ is robust at ultra-low thickness with a 330% magnetocurrent at 1.3 eV and room temperature for a 0.7 nm thick $Fe_2$ electrode (i.e., for 5 Fe atomic planes); (ii) $MC_{180}$ is only weakly thickness-dependent with a −25% relative variation while decreasing $Fe_2$ thickness from 1.7 nm down to 0.7 nm. The observed $MC_{180}$ reduction at low $Fe_2$ thickness is partially explained by thermal magnetization fluctuations which can be important at room temperature for epitaxial Fe deposited on Au(001).[18] From these observations, we deduce qualitatively that the magnetoconductance effects in our samples are dominated by interfacial rather than by volume spin-polarization effects. As a consequence, band structure matching at the interfaces of the heterostructure should be considered to justify the observed high magnetoconductance effects.

In similar simple Schottky contacts on GaAs, we have previously reported on the conservation of the hot-electron transverse momentum $k_{\parallel}$ while crossing epitaxial interface.[12] At low electron energy, close to the Schottky barrier height, electrons have access to the lowest valley of GaAs conduction band, which is located at the Γ point. This Γ-valley is projected on the $\bar{\Gamma}$ point of the two-dimensional Brillouin zone, i.e., around the $k_{\parallel} = 0$ direction. At higher energy, the GaAs conduction band presents also empty states in the L valley, so for $k_{\parallel}$ non-zero value. However, for a Fe/GaAs(001) Schottky contact, our previous study[12] demonstrated that the hot-electron transmission in this transverse valley is very weak. In the following analysis, based on ideas theoretically developed by Autès and co-workers for ballistic electrons at the Fermi energy in the Fe/Ag/Fe/InAs(001) spin-valve,[8] we will thus consider ballistic electron propagation around the $k_{\parallel} = 0$ direction only. Figure 2 displays the band structure of iron (for majority spin in red and for minority spin in black) and gold (in blue) in the $k_{\parallel} = 0$ direction (the so-called Δ direction). As the symmetry of the electron wave function should be conserved at each interface, because of the global symmetry of the heterostructure, above $\Phi_{SB}$, only majority electron states with $\Delta_1$ symmetry propagate in the iron layers. For iron minority spin, $\Delta_2$, $\Delta_2$, and $\Delta_5$ symmetry states are available in the probed energy range. In gold, available states have a $\Delta_1$ character only. Finally, the Γ valley of GaAs presents also a $\Delta_1$ symmetry. Due to the hot-electron wave function symmetry conservation, only $\Delta_1$ states of iron which are fully

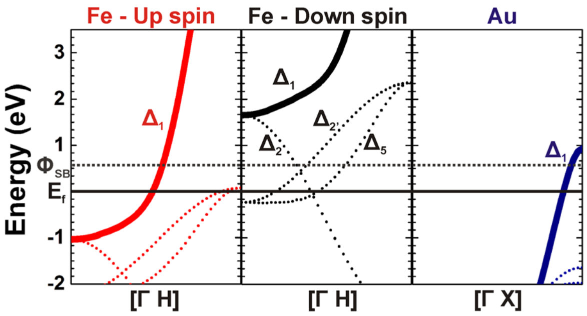


FIG. 2. Band structure along the $k_{\parallel} = 0$ direction for Fe majority spins (left, in red), for Fe minority spins (center, in black), and for Au (right, in blue). The horizontal continuous black line represents the Fermi energy and the horizontal dotted black line represents the Schottky barrier height ($\Phi_{SB} = 0.76$ eV) at the Fe/GaAs interface.

spin polarized for energy close to $\Phi_{SB}$ will be allowed to cross the Fe/Au interface. $\Delta_2$, $\Delta_2$, and $\Delta_5$ minority states will be totally reflected at this interface. This k-space spin-filtering effect induces a strong interfacial spin polarization of the hot-electron beam.

The previous analysis is rigorously valid for hot-electron states strictly collimated along the $k_{\parallel} = 0$ direction (i.e., at the GaAs $\bar{\Gamma}$ point). Away from this Δ high symmetry direction, the symmetry selection rules will be progressively released and the measured magnetocurrent should decrease while increasing the semiconductor collimator aperture. This is what is qualitatively observed on GaAs(001): the magnetocurrent amplitude is maximum close to $\Phi_{SB}$ and is decreasing at higher energy (see Figure 1(b)) when electrons can probe empty states with larger transverse momentum in the Γ valley of GaAs. Another fingerprint of the k-space spin filtering effect can also be evidenced by investigating the magnetocurrent dependence versus the effective mass m* of the semiconducting drain. The semiconductor collimator radius $k_{\parallel}^{max}$ is indeed scaling like $(m^*)^{1/2}$. We have also investigated three identical Au(2.2 nm)/Fe(1 nm)/Au(2.6 nm)/Fe(1.2 nm)/$Al_xGa_{1-x}As$(25 nm)/GaAs(001) spin-valves with various aluminium contents x = 0, 0.2, 0.4 in the semiconductor lead. The 25 nm thick $Al_xGa_{1-x}As$ layer was terminated by 4 atomic layers of GaAs in order to keep the Fe/semiconductor interface unchanged for all investigated heterostructures, and the $Fe_2$ thickness was set to 1 nm in order to obtain a 0°–180° variation of the relative angle $\theta$ between $Fe_1$ and $Fe_2$ magnetizations under magnetic field (see above). The Schottky barrier measured by BEMM and confirmed by classical current and capacitance versus voltage macroscopic measurements on these samples is $\Phi_{SB} = 0.76$ eV, 0.92 eV, and 1.05 eV for x = 0, 0.2, 0.4, respectively. In $Al_xGa_{1-x}As$ ternary alloys, the effective mass value and the energy positions of the different conduction band valleys are well known to evolve[19] with aluminium concentration x. For x = 0, 0.2, 0.4, the effective mass for the semiconductor conduction band minimum is $m^* = 0.067\ m_0$, $0.075\ m_0$, $0.226\ m_0$, respectively, $m_0$ being the free electron mass. Note that for $Al_{0.4}Ga_{0.6}As$, the first minimum of the conduction band is no longer the Γ valley but the X valley which is also projecting at the $\bar{\Gamma}$ point. The magnetocurrent amplitudes measured at 1.25 eV above the Fermi energy of the spin-valve for the three $Al_xGa_{1-x}As$ alloys are listed in the table of the inset of Figure 3(a). As expected, the magnetocurrent value for the same spin-valve is significantly dependent on the semiconductor lead effective mass and is decreasing from 380% for GaAs down to 286% for $Al_{0.4}Ga_{0.6}As$. This experimental dependence is coherent when the magnetocurrent is plotted versus the collimator aperture $k_{\parallel}^{max}$ at 1.25 eV ($k_{\parallel}^{max}$ is given in unit of the $\overline{\Gamma X}$ distance in the projected Brillouin zone, see sketch of Figures 3(b)–3(d)). In GaAs and $Al_{0.2}Ga_{0.8}As$, the experimental magnetocurrent amplitudes are identical at 1.25 eV, due to an identical collimator diameter $k_{\parallel}^{max} = 0.15^*\overline{\Gamma X}$ at this energy for both semiconductors.[20] In $Al_{0.4}Ga_{0.6}As$, collimator diameter increases to $k_{\parallel}^{max} = 0.2^*\overline{\Gamma X}$ at 1.25 eV, the efficiency of the electron angular filtering in the semiconductor around the $k_{\parallel} = 0$ direction is decreased and the magnetocurrent falls down to 286%.

This article is copyrighted as indicated in the abstract. Reuse of AIP content is subject to the terms at: http://scitation.aip.org/termsconditions. Downloaded to IP: 129.20.76.104 On: Wed, 20 Nov 2013 10:07:47

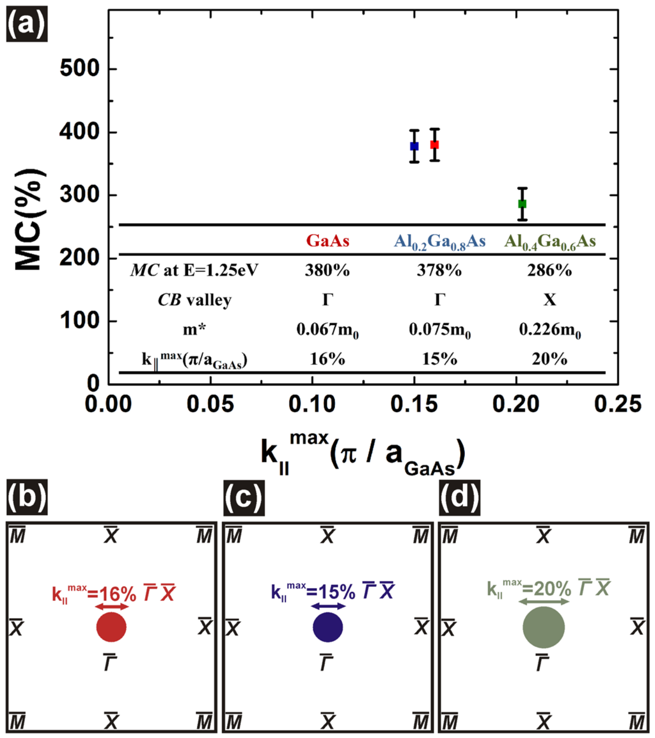


FIG. 3. (a) Evolution of the magnetocurrent amplitude at 1.25 eV versus maximum aperture in the semiconductor collimator for three Au(2.2 nm)/Fe(0.7–1.7 nm)/Au(2.6 nm)/Fe(1.2 nm)/$Al_xGa_{1-x}As$(25 nm)/GaAs(001) spin-valves with various aluminium contents x = 0, 0.2, 0.4. The inset table gives for the three samples the CB minimum probed close to the Schottky barrier, the corresponding effective mass m*, and collimator aperture $k_{\parallel}^{max}$ calculated at 1.25 eV. Sketch of the collimator aperture at 1.25 eV in the projected semiconductor 2D Brillouin zone of $Al_xGa_{1-x}As$ for x = 0 (b), x = 0.2 (c), and x = 0.4 (d).

To conclude, we have evidenced by ballistic electron magnetic microscopy large magnetoconductance effects in epitaxial Fe/Au/Fe/GaAs(001) epitaxial spin valves. These effects are robust in the ultrathin limit of the ferromagnetic electrodes pointing out an important contribution of the interfaces to the hot-electron spin-polarization mechanisms. We have also observed a strong dependence of the magnetocurrent amplitude with the semiconductor effective mass while replacing GaAs with $Al_xGa_{1-x}As$ alloys. These results support a dominant k-space spin-filtering effect in these ultrathin epitaxial spin-valves.[8] The semiconductor filters electrons with a momentum close to the $k_{\parallel} = 0$ direction and acts as a collimator. In this high symmetry direction of the spin-valve, the band structure matching at the Fe/Au interface selects $\Delta_1$ symmetry states which are fully spin polarized and the sample's conductance vanishes in the antiparallel magnetic configuration. This study opens the way to room-temperature ultra-high magnetoresistance values in designed epitaxial spin-valve deposited on semiconductor drain. Due to its low signal-to-noise ratio, BEMM does not allow a precise investigation of the magnetocurrent evolution in the immediate vicinity of $\Phi_{SB}$ where the largest effects are expected. Magnetotransport experiments on similar spin-valves with an integrated solid-state tunnel injector should thus be useful for a further quantitative investigation and deeper understanding of this k-space spin-filtering effect. This work is under progress.

This work was financially supported by Région Bretagne and Rennes Métropole. We warmly thank Andrey Umersky for enlightening discussions on the k-space spin-filtering effect. Technical support by Arnaud Le Pottier during the BEMM setup development is also gratefully acknowledged.

[1]M. Bowen, V. Cros, F. Petroff, A. Fert, C. M. Boubeta, J. L. Costa-Krämer, J. V. Anguita, A. Cebollada, F. Briones, J. M. de Teresa, L. Morellón, M. R. Ibarra, F. Güell, F. Peiró, and A. Cornet, Appl. Phys. Lett. **79**, 1655 (2001).
[2]J. Faure-Vincent, C. Tiusan, E. Jouguelet, F. Canet, M. Sajieddine, C. Bellouard, E. Popova, M. Hehn, F. Montaigne, and A. Schuhl, Appl. Phys. Lett. **82**, 4507 (2003).
[3]S. S. P. Parkin, C. Kaiser, A. Panchula, P. M. Rice, B. Hughes, M. Samant, and S. H. Yang, Nature Mater. **3**, 862 (2004).
[4]S. Yuasa, T. Nagahama, A. Fukushima, Y. Suzuki, and K. Ando, Nature Mater. **3**, 868 (2004).
[5]C. Chappert, A. Fert, and F. N. V. Dau, Nature Mater. **6**, 813 (2007).
[6]J. Mathon and A. Umerski, Phys. Rev. B **63**, 220403 (2001).
[7]W. H. Butler, X. G. Zhang, T. C. Schulthess, and J. M. MacLaren, Phys. Rev. B **63**, 054416 (2001).
[8]G. Autès, J. Mathon, and A. Umerski, Phys. Rev. B **83**, 052403 (2011).
[9]M. Hervé, S. Tricot, S. Guézo, G. Delhaye, B. Lépine, P. Schieffer, and P. Turban, J. Appl. Phys. **113**, 233909 (2013).
[10]W. H. Rippard and R. A. Buhrman, Appl. Phys. Lett. **75**, 1001 (1999).
[11]W. H. Rippard, A. C. Perrella, P. Chalsani, F. J. Albert, J. A. Katine, and R. A. Buhrman, Appl. Phys. Lett. **77**, 1357 (2000).
[12]S. Guézo, P. Turban, S. Di Matteo, P. Schieffer, S. Le Gall, B. Lépine, C. Lallaizon, and G. Jézéquel, Phys. Rev. B **81**, 085319 (2010).
[13]Y. Lu, D. Lacour, G. Lengaigne, S. Le Gall, S. Suire, F. Montaigne, and M. Hehn, Appl. Phys. Lett. **103**, 022407 (2013).
[14]W. H. Rippard and R. A. Buhrman, Phys. Rev. Lett. **84**, 971 (2000).
[15]O. Thomas, Q. Shen, P. Schieffer, N. Tournerie, and B. Lépine, Phys. Rev. Lett. **90**, 017205 (2003).
[16]M. Brockmann, S. Miethaner, R. Onderka, M. Köhler, F. Himmelhuber, H. Regensburger, F. Bensch, T. Schweinböck, and G. Bayreuther, J. Appl. Phys. **81**, 5047 (1997).
[17]E. Y. Tsymbal and D. G. Pettifor, Solid State Phys. **56**, 113 (2001).
[18]At 300 K, the saturation magnetization $M_S$ of a 1.7 nm Fe(001) film on Au(001) is $M_s = 0.9\ M_s^{bulk}$ and decreases to $M_s = 0.85\ M_s^{bulk}$ at 0.7 nm, $M_s^{bulk}$ being the saturation magnetization of bulk iron at 10 K, see W. Kipferl, M. Sperl, T. Hagler, R. Meier, and G. Bayreuther, J. Appl. Phys. **97**, 10B313 (2005).
[19]I. Vurgaftman, J. R. Meyer, and L. R. Ram-Mohan, J. Appl. Phys. **89**, 5815 (2001).
[20]The effective mass is larger in $Al_{0.2}Ga_{0.8}As$ than in GaAs but the conduction band minimum is also higher by 0.16 eV leading to the same $k_{\parallel}^{max}$ value.

This article is copyrighted as indicated in the abstract. Reuse of AIP content is subject to the terms at: http://scitation.aip.org/termsconditions. Downloaded to IP: 129.20.76.104 On: Wed, 20 Nov 2013 10:07:47
